# Supplementary material for: Caching for the Future: Scrub Jay Episodic Memory Principles for Agent Memory Systems
Source: arXiv:2608.04746 source file (2026-08-05)
Supplement: Supplementary file 1 [file appendix_iaa.tex]

% =============================================================================
% Appendix E — Human Inter-Annotator Agreement on TGT
% (run by tools/iaa_sample.py + tools/iaa_score.py; numbers in tab:tgt-iaa)
% =============================================================================
\section{Human Inter-Annotator Agreement on TGT}
\label{app:tgt-iaa}

To gauge whether the LLM judge (\texttt{llama3.2:3b}) used
throughout \S\ref{sec:e3-tgt} agrees with human assessors on the
two binary fields it labels (\texttt{factual\_correct},
\texttt{staleness\_aware}), we ran an inter-annotator agreement (IAA)
study over a stratified sample of $N=100$ (query, system-answer)
pairs drawn from the released TGT benchmark.

\paragraph{Sample.}
The sample was drawn by \texttt{tools/iaa\_sample.py} (seed $17$),
stratified across the four perishability classes and five retention
intervals ($5$ items per type-by-interval cell, $20$ cells $\times$
$5 = 100$ items). The blind annotation CSV exposed the query text,
the system's answer, the target-memory text, the ground-truth answer,
and the validity flag $\mathrm{ground\_truth\_valid}$ for that
session; the LLM judge's verdicts were withheld from annotators and
held by the keys file for scoring.

\paragraph{Annotators and protocol.}
Two human annotators (the paper authors) independently labelled each
sampled pair on the two binary fields exactly as the judge does:
$\texttt{factual\_correct} \in \{0,1\}$ (does the system's answer
contain the ground-truth attribute value?) and
$\texttt{staleness\_aware} \in \{0,1\}$ (is the system's validity
treatment consistent with the type$\times$interval schedule of
\Cref{tab:tgt-validity}?). Annotators did not see one another's
labels nor the LLM judge's labels during annotation.

\paragraph{Metrics.}
We report (a) raw percent agreement of each human rater against the
LLM judge, (b) Cohen's kappa of each human rater against the LLM
judge, (c) pairwise human--human percent agreement and Cohen's kappa,
and (d) Fleiss' kappa across the two human raters. Pre-registered
acceptance thresholds: $>$\,$90\%$ agreement on staleness; $>$\,$85\%$
on factual correctness; Cohen's kappa $\geq 0.6$ on both dimensions
(``substantial'' agreement by the Landis--Koch scale).

\paragraph{Results.}
\Cref{tab:tgt-iaa} summarises the run.

\begin{table*}[h]
  \centering
  \small
  \caption{TGT human IAA against the LLM judge and across human raters.
    $N=100$ stratified samples. Targets: $>$\,90\% / $>$\,85\%
    agreement on staleness / factual; Cohen's kappa $\geq 0.6$.
    \textbf{[Fill from \texttt{iaa\_score.py} output before submission.]}}
  \label{tab:tgt-iaa}
  \begin{tabular}{lcccc}
    \toprule
    Comparison & Dimension & \% agreement & Cohen's $\kappa$ & $n$ \\
    \midrule
    Rater A vs LLM judge   & factual\_correct  & [TBD] & [TBD] & 100 \\
    Rater A vs LLM judge   & staleness\_aware  & [TBD] & [TBD] & 100 \\
    Rater B vs LLM judge   & factual\_correct  & [TBD] & [TBD] & 100 \\
    Rater B vs LLM judge   & staleness\_aware  & [TBD] & [TBD] & 100 \\
    \midrule
    Rater A vs Rater B     & factual\_correct  & [TBD] & [TBD] & 100 \\
    Rater A vs Rater B     & staleness\_aware  & [TBD] & [TBD] & 100 \\
    \midrule
    Fleiss' $\kappa$       & factual\_correct  & n/a   & [TBD] & 100 \\
    Fleiss' $\kappa$       & staleness\_aware  & n/a   & [TBD] & 100 \\
    \bottomrule
  \end{tabular}
\end{table*}

\paragraph{Interpretation.}
% Fill once numbers are in. Suggested template:
% If thresholds are met: "Both Cohen's kappa values exceed 0.6 and
% raw agreement exceeds the pre-registered targets, supporting the
% use of the LLM judge as a proxy for human assessment on this task."
% If a threshold is missed: name the dimension that missed, the size
% of the gap, the most common disagreement mode (from the per-cell
% breakdown in iaa_score.py output), and what it implies for the
% magnitude of the GenGap claim.
\textbf{[Fill once the scoring run is complete. See
\texttt{iaa\_score.py} per-cell output to identify which (type,
interval) cells drove any disagreement.]}

\paragraph{Disagreement analysis.}
% Optional but recommended. Pull from `notes_optional` column +
% per-cell kappa breakdown. Common patterns:
%   - LLM judge marks staleness_aware=1 when the system hedges
%     ("I'm not sure") on an I3/I4 query for a Type-C memory.
%   - LLM judge accepts paraphrastic factual answers that humans
%     would reject (or vice versa) on factual_recall queries.
% Document any pattern that materially affects the headline metric.
\textbf{[Fill from \texttt{notes\_optional} column and per-cell
breakdown.]}

\paragraph{Reproducing this study.}
\begin{verbatim}
python tools/iaa_sample.py \
    --benchmark .benchmarks/e3_tgt_cache/tgt_benchmark.json \
    --predictions <path>/predictions/e3_tgt.jsonl \
    --system sjmem_full --n 100 --seed 17 \
    --out tools/iaa_out/tgt_iaa_sample

# Annotators each fill tgt_iaa_sample.blind.csv -> alice.csv, bob.csv
python tools/iaa_score.py \
    --keys  tools/iaa_out/tgt_iaa_sample.keys.json \
    --rater alice tools/iaa_out/alice.csv \
    --rater bob   tools/iaa_out/bob.csv \
    --report tools/iaa_out/tgt_iaa_report.json
\end{verbatim}
